# Supplementary material for: Untangling the Raman spectrum of cubic and tetragonal BaZrO$_3$
Source: arXiv:2409.16161 ancillary file (2024-12-17)
Supplement: Supplementary file 1 [file supporting-information.pdf]

# Supporting Information:

# Untangling the Raman spectrum of cubic and tetragonal $BaZrO_3$

Petter Rosander[1], Erik Fransson[1], Nicklas Österbacka[1], Paul Erhart[1], and Göran Wahnström[1]

[1] *Department of Physics, Chalmers University of Technology, SE-41296, Gothenburg, Sweden*

December 17, 2024

# Contents

**S1 Raman spectra** **2**
S1.1 Parallel and crossed spectra . . . . . 2
S1.2 Central Raman peak . . . . . 2
S1.3 Quantum corrections . . . . . 3

**S2 Phonon mode projections** **5**
S2.1 Mode coordinate . . . . . 5
S2.2 Time correlation function . . . . . 6
S2.3 Power spectrum . . . . . 7

**S3 Brownian dynamics** **8**
S3.1 Damped harmonic oscillator . . . . . 8
S3.2 Position dependent damping . . . . . 9
S3.3 Damped Morse oscillator . . . . . 10

# S1 Raman spectra

## S1.1 Parallel and crossed spectra

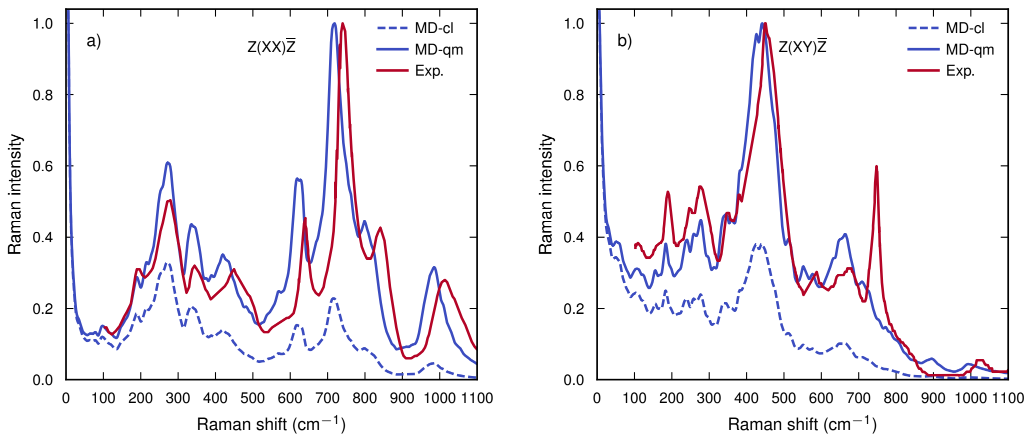


Figure S1: a) Parallel and b) crossed Raman spectra of $BaZrO_3$ at 300 K and 0 GPa. In the crossed Raman spectra there is a peak at 750 cm$^{-1}$ in the experimental data, which is not present in the theoretical data. The origin may be due to that in the experimental setup the crystal is not perfectly aligned and in that way some signal from the parallel configuration (which has a peak around 750 cm$^{-1}$) shows up in the crossed experimental data.

## S1.2 Central Raman peak

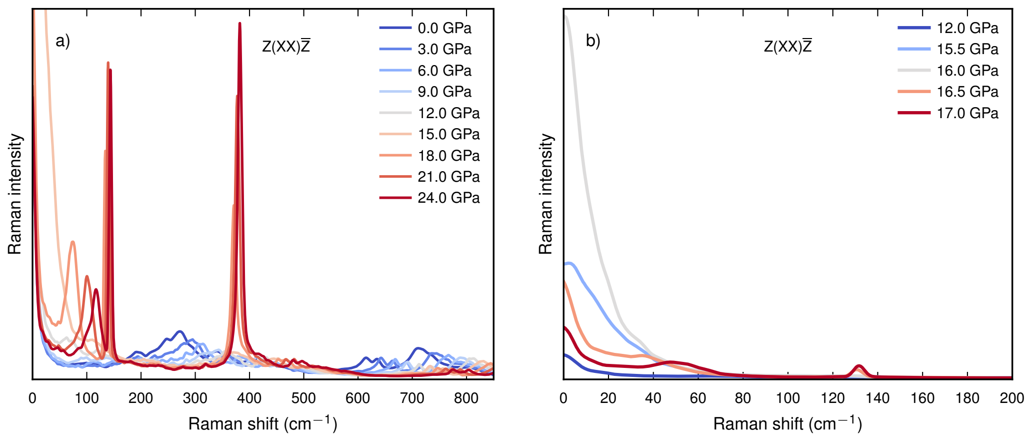


Figure S2: Parallel Raman spectra of $BaZrO_3$ at 300 K and at different pressures. a) Spectra at 0-24 GPa with 3 GPa increments. At 15 GPa a pronounced central peak is visible. b) Spectra at 12.0, 15.5, 16.0, 16.5 and 17.0 GPa. The phase transition to the tetragonal phase occurs at about 16.2 GPa.

## S1.3 Quantum corrections

Our calculation of the Raman spectra is based on MD simulations, *i.e.* on classical dynamics. Quantum dynamics will influence the results, renormalize phonons, and change the occupancy of phonon modes. The most important thing is to take the quantum statistics, the occupancy of the modes, into account. Even at room temperature, this effect can be large.

For a system described by a harmonic Hamiltonian, this can be done exactly. Following Cardona [1] the Raman intensity for first-order Stokes-Raman scattering in a harmonic crystal can be written as

$$I_{\mathrm{qm}}(\omega) = \frac{V}{(4\pi)^2}\frac{\omega_s^4}{c^4} \mid \mathbf{e}_s \cdot \frac{d\chi}{d\xi} \cdot \mathbf{e}_L \mid^2 \; S_{\mathrm{qm}} \tag{S1}$$

where the statistical factor $S_{\mathrm{qm}}$ is given by

$$S_{\mathrm{qm}} = \langle \xi\xi^\dagger \rangle = \sum_k \langle n|\xi|k\rangle \langle k|\xi^\dagger|n\rangle = | \langle n+1|\xi^\dagger|n\rangle |^2 = \frac{\hbar}{2\omega}\left[n(\omega)+1\right] \tag{S2}$$

and where $\xi^\dagger$ and $\xi$ are the phonon creation and annihilation operators, respectively, and

$$n(\omega) = \frac{1}{\exp(\beta\hbar\omega)-1} \tag{S3}$$

is the Bose-Einstein occupation factor. It is the statistical factor $S_{\mathrm{qm}}$ that incorporates the proper quantum fluctuations in the system. In the classical limit it reduces to

$$S_{\mathrm{cl}} = \frac{1}{2\beta\omega^2} \tag{S4}$$

A computed Raman intensity based on classical mechanics $I_{cl}(\omega)$ can then be used to obtain the true Raman intensity based on quantum mechanics according to

$$I_{\mathrm{qm}}(\omega) = \frac{S_{\mathrm{qm}}}{S_{\mathrm{cl}}}\; I_{\mathrm{cl}}(\omega) = \frac{\beta\hbar\omega}{1-\exp(-\beta\hbar\omega)} I_{\mathrm{cl}}(\omega) \tag{S5}$$

Consider now second-order Stokes-Raman scattering. Then we can distinguish between scattering by two of the same phonons (overtones) and by two different phonons (combinations). In the latter

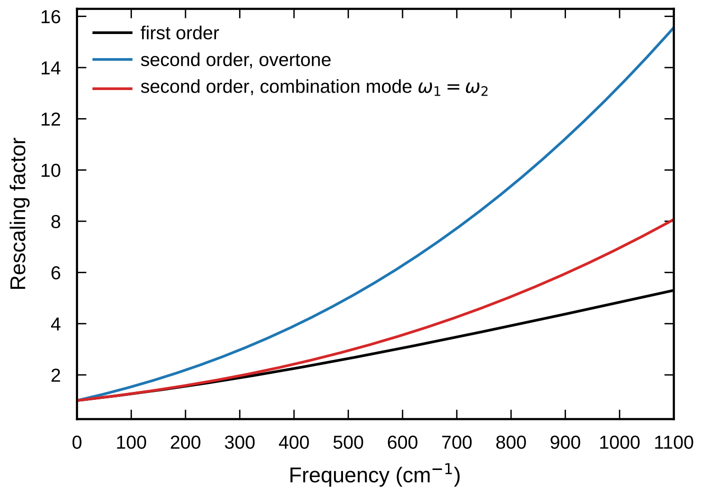


Figure S3: Rescaling factor $S_{\mathrm{qm}}/S_{\mathrm{cl}}$ at T = 300 K as function of frequency $\omega$. Black curve: first order scattering (see Eq. S5); Blue curve: second order scattering, overtone (see Eq. S7); Red curve: second order scattering, combination mode with $\omega_1 = \omega_2$ (see Eq. S10).

case, differences are also possible. For overtones with frequency $\omega_1$ we have that [1]

$$S_{\rm qm} = \frac{\hbar}{2\omega_1}[n(\omega_1)+1]\ \frac{\hbar}{2\omega_1}[n(\omega_1)+2] \tag{S6}$$

with $\omega_1 = \omega/2$. The quantum mechanical intensity can then be obtain as

$$I_{\rm qm}(\omega) = \left(\frac{\beta\hbar\omega/2}{1-\exp\left(-\beta\hbar\omega/2\right)}\right)^2 \left[2-\exp\left(-\beta\hbar\omega/2\right)\right]\ I_{\rm cl}(\omega) \tag{S7}$$

using a computed classical intensity $I_{\rm cl}(\omega)$.

For a combination mode with frequencies $\omega_1$ and $\omega_2$ we have that [1]

$$S_{\rm qm} = \frac{\hbar}{2\omega_1}[n(\omega_1)+1]\ \frac{\hbar}{2\omega_2}[n(\omega_2)+1] \tag{S8}$$

with $\omega_1 + \omega_2 = \omega$. The quantum mechanical intensity can then be obtain as

$$I_{\rm qm}(\omega) = \frac{\beta\hbar\omega_1}{1-\exp\left(-\beta\hbar\omega_1\right)}\ \frac{\beta\hbar\omega_2}{1-\exp\left(-\beta\hbar\omega_2\right)}\ I_{\rm cl}(\omega) \tag{S9}$$

using a computed classical intensity $I_{\rm cl}(\omega)$. The largest quantum correction for a combination mode is obtained assuming $\omega_1 = \omega_2$, i.e.

$$I_{\rm qm}(\omega) = \left(\frac{\beta\hbar\omega/2}{1-\exp\left(-\beta\hbar\omega/2\right)}\right)^2 I_{\rm cl}(\omega)\ . \tag{S10}$$

while the smallest quantum correction for a combination mode is obtained assuming $\omega_1 = \omega$ (and hence $\omega_2 = 0$) or $\omega_2 = \omega$ (and hence $\omega_1 = 0$). The result is then given by Eq. S5. For an arbitrary combination mode, the result will be between the black and red curves in Fig. S3.

# S2 Phonon mode projections

## S2.1 Mode coordinate

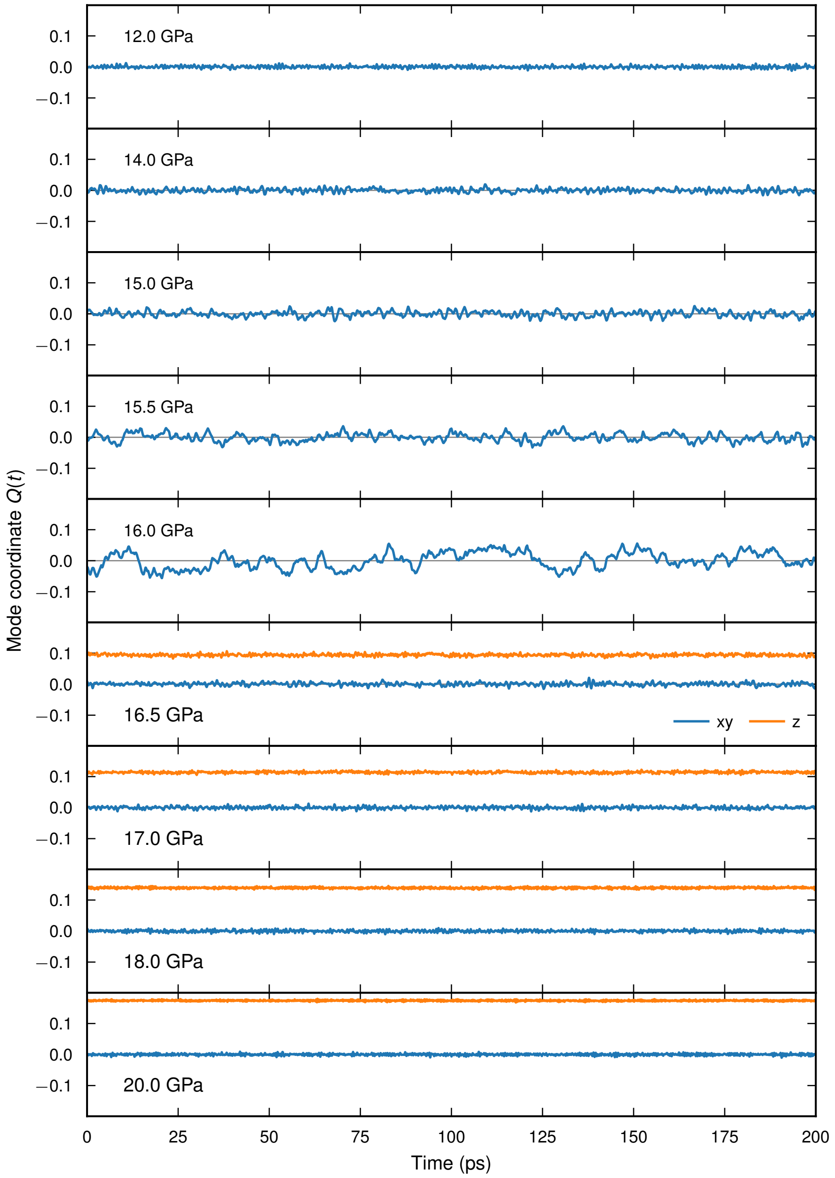


Figure S4: Time dependence of the phonon mode coordinate $Q_\lambda(t) = \langle\, \mathbf{e}_\lambda \mid \mathbf{u}(t)\, \rangle$.

## S2.2 Time correlation function

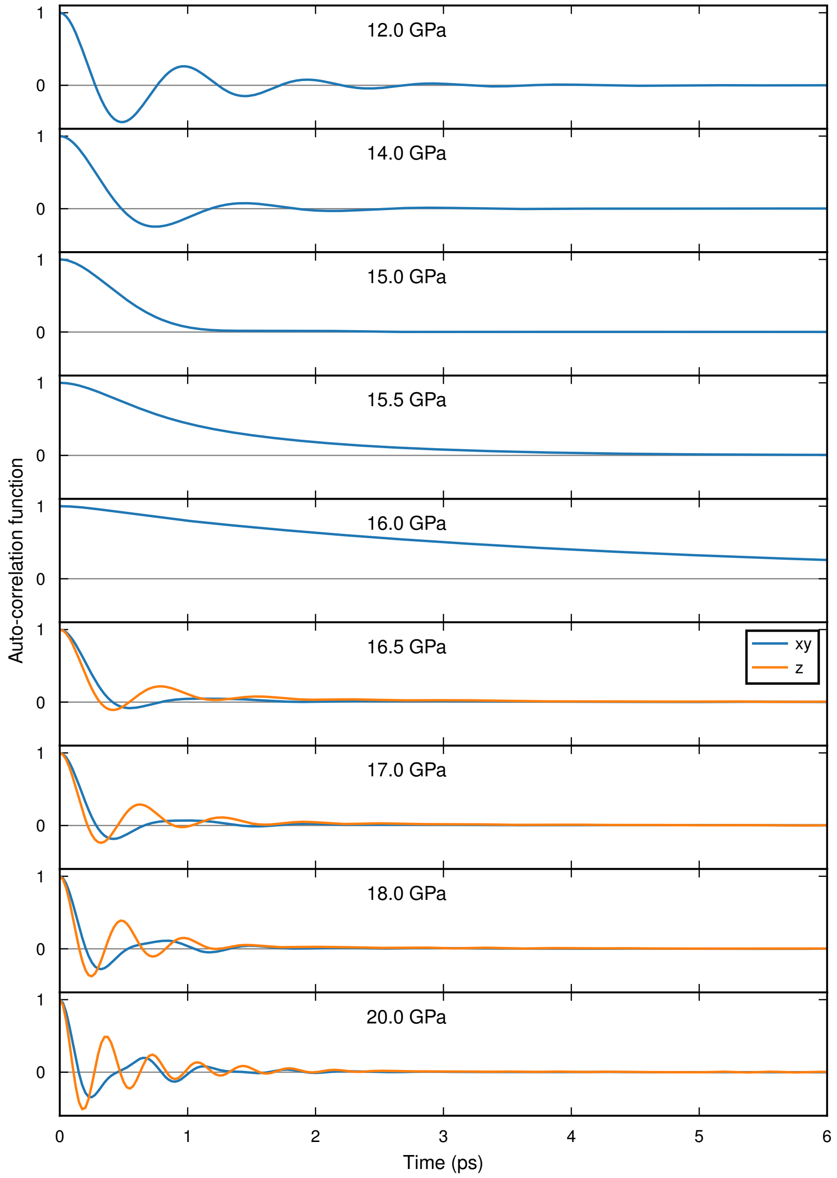


Figure S5: The phonon mode time correlation function $C(t) = \langle Q_\lambda(t+t')Q_\lambda(t')\rangle$.

## S2.3 Power spectrum

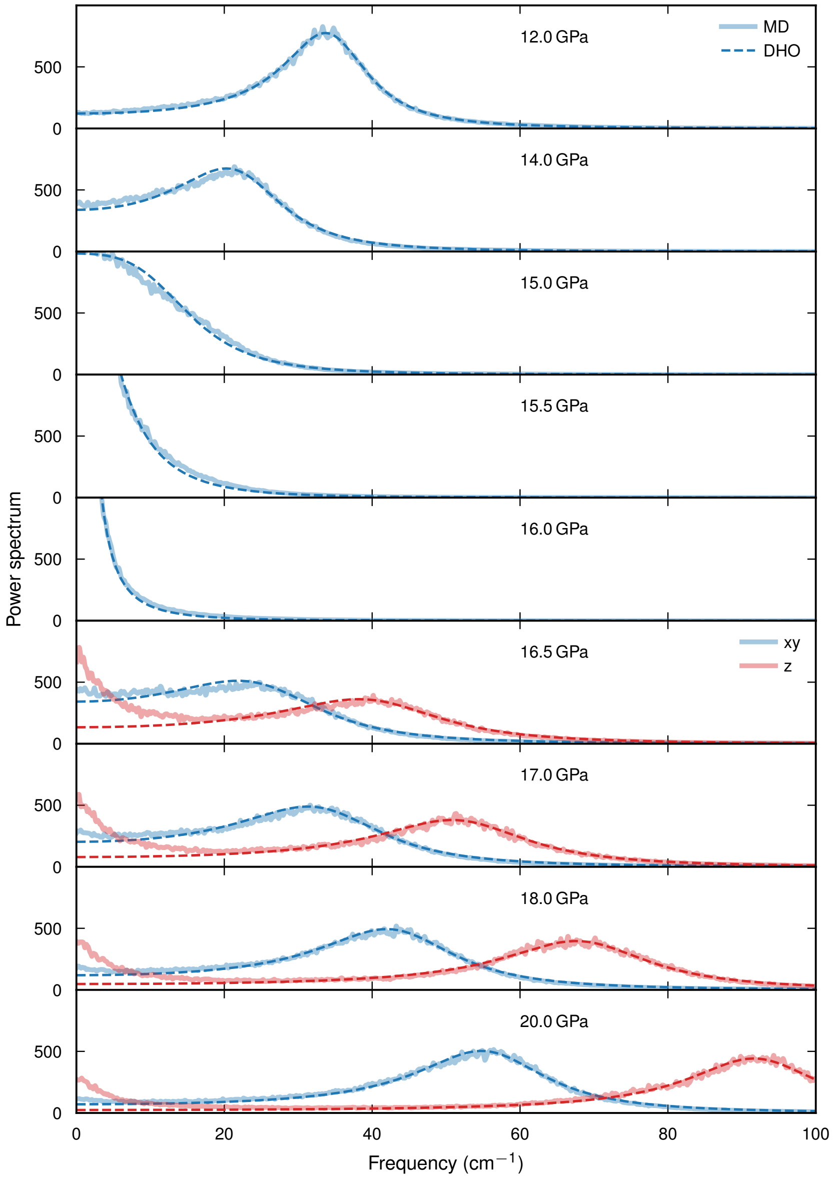


Figure S6: Power spectrum of the phonon mode coordinate $P(\omega) = \int \mathrm{d}t\, e^{-i\omega t} C(t)$.

# S3 Brownian dynamics

## S3.1 Damped harmonic oscillator

The time evolution of the phonon mode coordinate $Q(t)$ can be modelled as the motion of a damped harmonic oscillator (DHO) with the natural frequency $\omega_0$ and damping $\Gamma$ according to

$$\ddot{Q}(t) + \omega_0^2\, Q(t) = -\Gamma\, \dot{Q}(t) + \xi^{\mathrm{st}}(t)\ , \tag{S11}$$

where $\xi^{\mathrm{st}}(t)$ is a fluctuating force with white noise spectrum

$$\langle \xi^{\mathrm{st}}(t)\xi^{\mathrm{st}}(t')\rangle = 2\Gamma k_{\mathrm{B}} T \delta(t-t'). \tag{S12}$$

and where $\langle \ldots \rangle$ denotes a time average. The auto-correlation function for the phonon mode coordinate, $C(t) \equiv \langle Q(t+t')Q(t')\rangle$, is then given by the equation

$$\ddot{C}(t) + \Gamma\, \dot{C}(t) + \omega_0^2\, C(t) = 0 \tag{S13}$$

with $C(0) = k_{\mathrm{B}}T/\omega_0^2$ and $\dot{C}(0) = 0$. The solution to Eq. S13 in time splits into an underdamped regime ($\omega_0 > \Gamma/2$) with a damped oscillatory motion and an overdamped regime ($\omega_0 < \Gamma/2$) with an exponential decay in time [2]. The corresponding power spectrum is given by

$$P(\omega) = k_{\mathrm{B}} T \frac{2\,\Gamma}{(\omega^2 - \omega_0^2)^2 + (\Gamma\omega)^2}\ . \tag{S14}$$

For frequencies $\omega_0 > \Gamma/\sqrt{2}$ the spectrum exhibits a peak with peak position $\omega_p = \sqrt{\omega_0^2 - \Gamma^2/2}$ , while for $\omega_0 < \Gamma/\sqrt{2}$ the spectrum only shows a central peak, which approaches a Lorentzian with the half width at half maximum equal to $\omega_0^2/\Gamma$ when $\omega_0/\Gamma$ decreases.

### Example

Consider now a harmonic oscillator with the natural frequency $\omega_0 = 1.2\,\mathrm{ps}^{-1}$ ($\omega_0 = 40\,\mathrm{cm}^{-1}$) at temperature $T = 300\,\mathrm{K}$. We consider two different values of the damping: $\Gamma = 0.2\,\mathrm{ps}^{-1}$ and $\Gamma = 2.6\,\mathrm{ps}^{-1}$. The former corresponds to low damping $\Gamma/2 < \omega_0$, while the latter corresponds to high damping $\Gamma/2 > \omega_0$. As seen in Fig. S7, the distribution of the phonon mode coordinate is the same in the two different cases while the power spectra differ. At low damping an oscillatory peak is visible, whereas at high damping only a central peak appears in the spectrum.

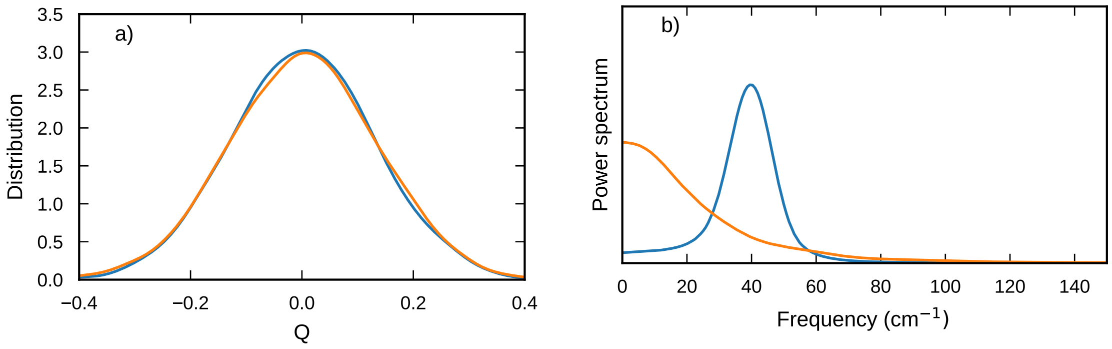


Figure S7: Results for the DHO potential with low damping $\Gamma/2 < \omega_0$ (blue curve) and high damping $\Gamma/2 > \omega_0$ (red curve). a) The distribution of the oscillator. b) The power spectrum of the solution.

## S3.2 Position dependent damping

The extra peak in the spectrum for the $Q_z$-phonon mode coordinate in the tetragonal phase may be due to some asymmetry in the damping. If the damping is small in some region and large in some other region, the motion may contain both damped and overdamped oscillatory motion. Therefore, we extend the simple damped harmonic oscillator model in Eq. S11 by adding an asymmetric position dependent damping $\Gamma(Q)$, according to

$$\ddot{Q}(t) + \omega_0^2\, Q(t) = -\Gamma(Q)\, \dot{Q}(t) + \xi^{\rm st}(t, Q)\ , \tag{S15}$$

The fluctuating force also then become position dependent. This equation has to be solved numerically. We use the integrator for the Langevin equation introduced by Bussi and Parrinello [3]. For $\Gamma(Q)$ we assume the asymmetric form

$$\Gamma(Q) = \Gamma_0 + A\ \Theta(Q)\ Q^2.$$

where $\Theta(Q)$ is the Heaviside step function. The model then contains three parameters, the natural frequency $\omega_0$, the base damping $\Gamma_0$, and the damping strength parameter $A$.

### Example

Consider a system defined by the parameters $\omega_0 = 1.2\,\text{ps}^{-1}$, $\Gamma_0 = 0.2\,\text{ps}^{-1}$, and $A = 200\,\text{eV}^{-1}\text{ps}^{-3}$ at temperature $T = 300\,\text{K}$. In Fig. S8a we show the obtained distribution for the phonon mode coordinate, which is symmetric, together with the damping function $\Gamma(Q)$. The power spectrum in Fig. S8b consists of a central peak and a damped oscillatory peak around $40\,\text{cm}^{-1}$. This corresponds to $1.2\,\text{ps}^{-1}$ in nice agreement with $\omega_0$.

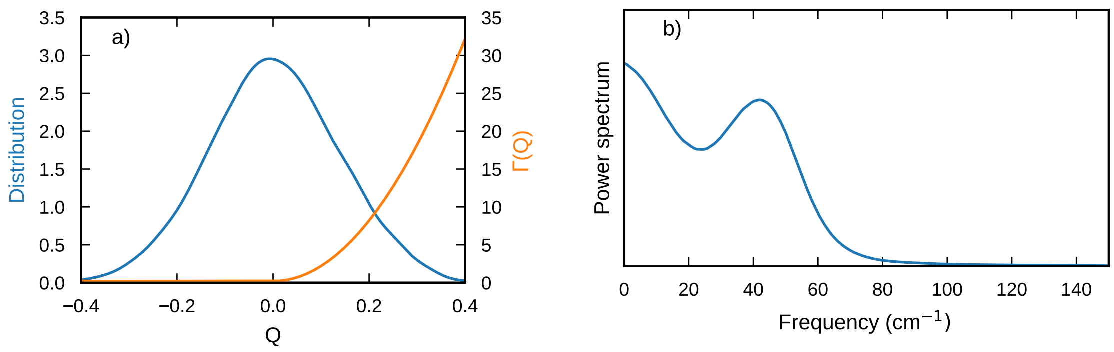


Figure S8: Results for the damped oscillator potential with a position dependent damping. a) The distribution of the oscillator together with the position dependent damping. b) Power spectrum of the solution.

## S3.3 Damped Morse oscillator

The harmonic potential is symmetric. Another possibility to obtain an asymmetry is to change the potential. Therefore, we consider the asymmetric Morse potential, defined as,

$$V(Q) = D(1 - e^{-\alpha Q})^2.$$

The force on the particle is then given by,

$$F(Q) = -2\alpha D \left(1 - e^{-\alpha Q}\right) e^{-\alpha Q}$$

and at small displacements, the oscillation frequency is equal to $\omega_{\text{min}} = \alpha\sqrt{2D}$. The equation of motion is then given by

$$\ddot{Q}(t) + 2\alpha D \left(1 - e^{-\alpha Q(t)}\right) e^{-\alpha Q(t)} = -\Gamma\dot{Q}(t) + \xi^{\text{st}}(t)$$

and is solved using the integrator introduced by Bussi and Parrinello [3]. The model contains three parameters, the damping $\Gamma$, and the two potential parameters $D$ and $\alpha$.

### Example

Consider a system defined by the parameters $D = 0.258\,\text{eV}$, $a = 4.2\,\text{eV}^{-1/2}\text{ps}^{-1}$, and $\Gamma = 0.08\,\text{ps}^{-1}$ and the temperature $T = 300\,\text{K}$. In Fig. S9a we show the obtained distribution for the phonon mode coordinate, together with the Morse potential. The distribution is asymmetric with a tail towards large values for $Q$. Ihe power spectrum in Fig. S9b consist of a large central peak and a damped oscillatory peak around $92\,\text{cm}^{-1}$. This can be compared with the frequency at the minimum, $\omega_{\text{min}}$, which is slightly higher, equal to $101\,\text{cm}^{-1}$. This is expected on the basis of the anharmonicity of the Morse potential.

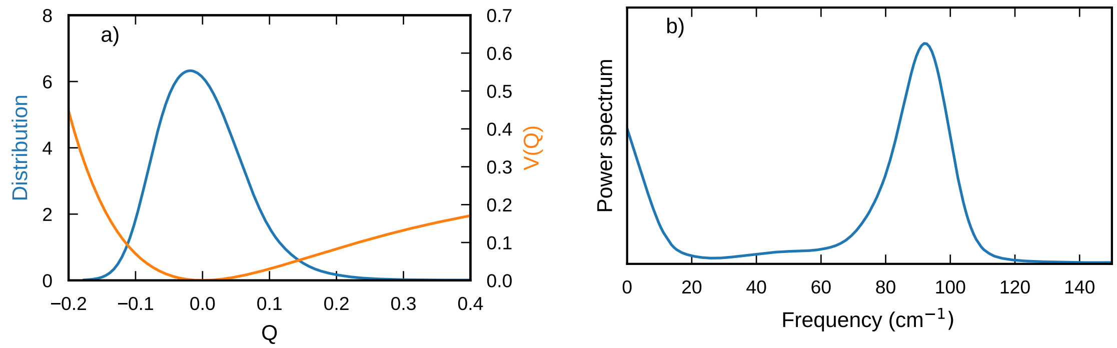


Figure S9: Results for the damped Morse oscillator. a) The distribution of the oscillator together with the Morse potential. b) Power spectrum of the solution.

# Supplemental References

[1] M. Cardona, *Resonance phenomena*, edited by M. Cardona and G. Güntherodt, in Topics in Applied Physics, Vol. 50 (Springer, 1982).

[2] E. Fransson, P. Rosander, F. Eriksson, J. M. Rahm, T. Tadano, and P. Erhart, Communications Physics **6**, 1–7 (2023).

[3] G. Bussi and M. Parrinello, Physical Review E **75**, 056707 (2007).
